# Supplementary material for: What do QAOA energies reveal about graphs?
Source: arXiv:1912.12277 source file (2019-12-31)
Supplement: Supplementary file 1 [file appendix.tex]

\section{APPENDIX}

We call a function of the form 
$F:\{0,1\}^{n}\rightarrow \mathbb{R}$ a {\em landscape} on $n$-bits.
An example to a landscape is ${\rm CUT}(G,z) = |G[z(0),z(1)]|$, where $z(0)$ and $z(1)$ are the zero- and one- sets of $z$, and 
$G[V_{1},V_{2}]$ represents the set of edges between $V_{1}$ and $V_{2}$ (so any $z\in \{0,1\}^{n}$ defines a cut).
We say that the two landscapes are {\em isomorphic} if there is an 
automorphism $\rho$ of the hypercube graph, $C_{n}$, such that 
for all $z\in \{0,1\}^{n}$ we have $F(\rho(z)) = F'(z)$. It is well known
that the automorphism group of the hypercube graph has size $2^{n}n!$ (see \cite{}), where 
the $n!$ part corresponds to permuting the $n$ labels and the $2^{n}$ part corresponds to 
automorphisms  of the form $\rho_{w}: z \rightarrow z \oplus w$. Alternatively,
the group can be explained as the wreath product ${\rm Aut}(C_{n}) = Z_{2}\wr S_{n}$.
The following lemma is not hard to prove:
\begin{lemma} \label{isos}
Let graphs $G$ and $G'$ be connected graphs on $n$ nodes. The following are
equivalent:
\begin{enumerate}
\item Landscapes ${\rm CUT}(G,z)$, ${\rm CUT}(G',z)$ are isomorphic.
\item Graphs $G$ and $G'$ are isomorphic.
\end{enumerate}
\end{lemma}

The lemma is proved in Appendix A. Unfortunately, for landscapes $F$ and $F'$ the equality $QAOA(F,\vec{\gamma},\vec{\beta}) = QAOA(F',\vec{\gamma},\vec{\beta})$,
even when holds for all angle sequences $(\vec{\gamma},\vec{\beta})$, does not imply that
$F$ and $F'$ are isomorphic. A counter-example is given in Appendix B.
This however does not rule out that the statement holds when $F$ and $F'$ are CUT functions of two graphs. Although this  would 
not put graph isomorphism into quantum polynomial time, because for that we would need quantitative bounds, but would at least rule out unwanted coincidences,
as \cite{} does in the context of a boson sampling approach.

A simple observation may help us in the future:
\begin{lemma}
Let $G$ and $G'$ be two non-isomorphic graphs and $F$ and $F'$ be their energy landscapes under MAXCUT. Then $|F-F'|_{1} \ge 1$, where 
the $L_{1}$ norm of an $F:\{0,1\}^{n}\rightarrow \mathbb{R}$ is defined as $|F|_{1} = {1\over 2^{n}} \sum_{z\in \{0,1\}^{n}} |F(z)|$.
\end{lemma}

The above lemma implies that if $G$ and $G'$ are non-isomorphic, then their corresponding landscapes are far from being 
weakly isomorphic. Let us now return to the proof of Lemma \ref{distinct}. We first write down 
\[
QAOA(F,\vec{\gamma},\vec{\beta}) = \sum \prod 
\]
